# Supplementary material for: Realizations of Indecomposable Persistence Modules of Arbitrarily Large Dimension
Source: arXiv:1803.05722 source file (2018-12-19)
Supplement: Supplementary file 1 [file 08_vr_appendix.tex]

\section{Details on the Vietoris-Rips construction for the commutative ladder}\label{sec:appendixVR}

We provide details to reproduce our Vietoris-Rips construction.
Every tile we consider is a planar point set contained within a square with sides of length $5$.
Coordinates for all the points in the various tiles are displayed in Table~\ref{tab:coordinates}.
Note that some points lie on the boundary of the tiles.
In assembling the global point sets $P_\ell$ and $P_u$, the tiles intersect only along the boundaries, where the points coincide.

\begin{table}[htb]
\caption{Coordinates of points within tiles.}\label{tab:coordinates}
\begin{center}
\begin{tabular}{|l|c|c|c|c|c|c|}
\hline
Index\textbackslash Tile & A & B & C & D & E & F \\ \hline
1 & (0, 0) & (0, 0) & (0, 0) & (0, 0) & (0, 0) & (0, 0)\\
2 & (0, 5) & (0, 5) & (0, 5) & (0, 5) & (0, 5) & (0, 5)\\
3 & (5, 5) & (5, 5) & (5, 5) & (5, 5) & (5, 5) & (5, 5)\\
4 & (5, 0) & (5, 0) & (5, 0) & (5, 0) & (5, 0) & (5, 0)\\ \hline
5 & (1.5, 0) & (1.3, 0) & (.7, 0) & (1.3 0) & (1.3, 0) & (.5, 0)\\
6 & (3.5, 0) & (3.7, 0) & (4.3, 0) & (3.7, 0) & (3.7, 0) & (4.5, 0)\\ \hline
7 & (1.5, 5) & (1.3, 5) & (1.5, 5) & (1.3, 5) & (1.3, 5) & (.7, 5)\\
8 & (3.5, 5) & (3.7, 5) & (3.5, 5) & (3.7, 5) & (3.7, 5) & (4.3, 5)\\ \hline
9 & (0, 1.5) & (0, 0.7) & (0, 1.5) & (0, 1.3) & (0, .5) & (0, 1.3) \\
10 & (0, 3.5) & (0, 4.3) & (0, 3.5) & (0, 3.7) & (0, 4.5) & (0, 3.7) \\ \hline
11 & (5, 0.7) & (5, 1.5) & (5, 1.5) & (5, .5) & (5, 1) & (5, 1.3)\\
12 & (5, 4.3) & (5, 3.5) & (5, 3.5) & (5, 4.5) & (5, 4) & (5, 3.7)\\ \hline
13 & (1.86, 2.5) & (3, 2.5) & (2.5, 2.9) & (2, 2.5) & (3, 2.5) & (2.5, 3.5) \\ \hline
\end{tabular}
\end{center}
\end{table}

After building the point sets, we set the radius parameters $r_i$ to be any value within the open intervals $(x_i,y_i)$, for each $i$, described in Table~\ref{tab:range}.

\begin{table}[htb]
\caption{Ranges for the choice of parameters.}\label{tab:range}
\begin{center}
\begin{tabular}{|l|c|c|c|c|c|}
\hline
Parameter & $r_1$ & $r_2$ & $r_3$ & $r_4$ & $r_5$ \\ \hline
$x_i$ & 1.06 & 1.21 & 1.6 & 1.8 & 2\\
$y_i$ & 1.12 & 1.25 & 1.665 & 1.805 & 2.015\\ \hline
\end{tabular}
\end{center}
\end{table}

Choosing radii inside these interval guarantees that the abstract Vietoris-Rips complex of the lower row is a subcomplex of the abstract Vietoris-Rips complex of the upper row.
It does not however guarantee the inclusion of their domains.
We provide below a geometric tilewise representation of theses complexes for the chosen radii.

\FloatBarrier
\begin{figure}[htb!]
  \caption{Tile A}
  \begin{center}
  \begin{tikzpicture}[scale=0.34]
    \Atile{0}{0}{0}{0}
    \Atile{7}{0}{0}{1}
    \Atile{14}{0}{0}{2}
    \Atile{21}{0}{0}{3}
    \Atile{28}{0}{0}{4}
    \Atile{35}{0}{0}{5}
  \end{tikzpicture}
\end{center}
\end{figure}

\begin{figure}[htb!]
  \caption{Tile B}
  \begin{center}
  \begin{tikzpicture}[scale=0.34]
    \Btile{0}{0}{0}{0}
    \Btile{7}{0}{0}{1}
    \Btile{14}{0}{0}{2}
    \Btile{21}{0}{0}{3}
    \Btile{28}{0}{0}{4}
    \Btile{35}{0}{0}{5}
  \end{tikzpicture}
\end{center}
\end{figure}

\begin{figure}[htb!]
  \caption{Tile C}
  \begin{center}
  \tdplotsetmaincoords{90}{270}
  \begin{tikzpicture}[scale=0.34, tdplot_main_coords]
    \Ctile{0}{35}{0}{0}
    \Ctile{0}{28}{0}{1}
    \Ctile{0}{21}{0}{2}
    \Ctile{0}{14}{0}{3}
    \Ctile{0}{7}{0}{4}
    \Ctile{0}{0}{0}{5}
  \end{tikzpicture}
\end{center}
\end{figure}

\begin{figure}[htb!]
  \caption{Tile D}
  \begin{center}
  \begin{tikzpicture}[scale=0.34]
    \Dtile{0}{0}{0}{0}
    \Dtile{7}{0}{0}{1}
    \Dtile{14}{0}{0}{2}
    \Dtile{21}{0}{0}{3}
    \Dtile{28}{0}{0}{4}
    \Dtile{35}{0}{0}{5}
  \end{tikzpicture}
\end{center}
\end{figure}

\begin{figure}[htb!]
  \caption{Tile E}
  \begin{center}
  \begin{tikzpicture}[scale=0.34]
    \Etile{0}{0}{0}{0}
    \Etile{7}{0}{0}{1}
    \Etile{14}{0}{0}{2}
    \Etile{21}{0}{0}{3}
    \Etile{28}{0}{0}{4}
    \Etile{35}{0}{0}{5}
  \end{tikzpicture}
\end{center}
\end{figure}

\begin{figure}[htb!]
  \caption{Tile E reversed}
  \begin{center}
  \begin{tikzpicture}[scale=0.34]
    \EtileR{0}{0}{0}{0}
    \EtileR{7}{0}{0}{1}
    \EtileR{14}{0}{0}{2}
    \EtileR{21}{0}{0}{3}
    \EtileR{28}{0}{0}{4}
    \EtileR{35}{0}{0}{5}
  \end{tikzpicture}
\end{center}
\end{figure}

\begin{figure}[htb!]
  \caption{Tile F}
  \begin{center}
  \tdplotsetmaincoords{90}{270}
  \begin{tikzpicture}[tdplot_main_coords,scale=0.34]
    \Ftile{0}{35}{0}{0}
    \Ftile{0}{28}{0}{1}
    \Ftile{0}{21}{0}{2}
    \Ftile{0}{14}{0}{3}
    \Ftile{0}{7}{0}{4}
    \Ftile{0}{0}{0}{5}
  \end{tikzpicture}
\end{center}
\end{figure}

\FloatBarrier

%%% Local Variables:
%%% mode: latex
%%% TeX-master: "jitsugen_journal"
%%% End:
